# Supplementary material for: Optimal local approximation spaces for parabolic problems
Source: arXiv:2012.02759 ancillary file (2021-08-24)
Supplement: Supplementary file 1 [file supplement.pdf]

# SUPPLEMENTARY MATERIALS: OPTIMAL LOCAL APPROXIMATION SPACES FOR PARABOLIC PROBLEMS

JULIA SCHLEUSS AND KATHRIN SMETANA

## SM1. Calculation corresponding to Remark 5.3

We assume that $I = (0,1)$ and $\Omega^{out} = (0,\pi)^2$ and consider the linear heat equation

$$\partial_t \tilde{u} - \Delta \tilde{u} = 0 \ \text{ in } I \times \Omega^{out}, \ \ \tilde{u}(0,x) = 0 \ \ \forall\, x \in \Omega^{out}, \ \ \tilde{u}(t,x) = t \ \ \forall\,(t,x) \in I \times \partial\Omega^{out}.$$

To compute the solution $\tilde{u}$, we define the auxiliary function $v(t,x) := \tilde{u}(t,x) - t$. Consequently, $v$ solves the equation

$$\partial_t v - \Delta v = -1 \ \text{ in } I \times \Omega^{out}, \ \ v(0,x) = 0 \ \ \forall\, x \in \Omega^{out}, \ \ v(t,x) = 0 \ \forall\,(t,x) \in I \times \partial\Omega^{out}.$$

We have that $v(t,x_1,x_2) = \sum_{k,l=1}^{\infty} v_{k,l}(t)\sin(kx_1)\sin(lx_2)$, where $v_{k,l}(0) = 0$. Using Fourier series we can conclude that

$$\begin{aligned}\sum_{k,l=1}^{\infty} ((v_{k,l})_t(t) + (k^2+l^2)v_{k,l}(t))\sin(kx_1)\sin(lx_2) &= -1 \\ &= \sum_{k,l=1}^{\infty} -\frac{4\,(1-\cos(k\pi))(1-\cos(l\pi))}{k\,l\,\pi^2}\sin(kx_1)\sin(lx_2).\end{aligned}$$

Solving the ordinary differential equation

$$(v_{k,l})_t(t) + (k^2+l^2)v_{k,l}(t) = -\frac{4\,(1-\cos(k\pi))(1-\cos(l\pi))}{(k\,l\,\pi^2)}, \quad v_{k,l}(0) = 0,$$

yields $v_{k,l}(t) = -4\,(1-\cos(k\pi))(1-\cos(l\pi))(1-e^{-(k^2+l^2)t})/(k\,l\,(k^2+l^2)\,\pi^2)$ and we thus have that

$$\tilde{u}(t,x_1,x_2) = \sum_{k,l=1}^{\infty} -\frac{4\,(1-\cos(k\pi))(1-\cos(l\pi))(1-e^{-(k^2+l^2)t})}{k\,l\,(k^2+l^2)\,\pi^2}\sin(kx_1)\sin(lx_2) + t.$$

Moreover, one can infer that $\hat{u}(t,x_1,x_2) = -\tilde{u}(t,x_1,x_2) + t$. Therefore, it holds that $\|\nabla(\tilde{u}+\hat{u})\|_{L^2(I,L^2(\Omega^{out}))} = 0$ while $\|\nabla\tilde{u}\|_{L^2(I,L^2(\Omega^{out}))} > 0$.

## SM2. Quasi-optimal local approximation spaces

In this section we outline how the optimal local spaces $\Lambda^n$ introduced in section 3 can be approximated via random sampling. For further details we refer to [SM2] where methods from randomized linear algebra [SM3] have been used to approximate the optimal local approximation spaces in the elliptic setting.

*Date*: December 4, 2020.

The work of Julia Schleuß was funded by the Deutsche Forschungsgemeinschaft (DFG, German Research Foundation) under Germany's Excellence Strategy EXC 2044-390685587, Mathematics Münster: Dynamics-Geometry-Structure.

**Algorithm 1:** Adaptive randomized local basis generation

1 **Function** `AdaptiveRandomizedLocalBasis`($P_h$,`tol`,$n_t$,$\varepsilon_{\text{algofail}}$)`:`

**Input :** transfer operator $P_h$ of rank $N_{P_h}$,
target accuracy `tol`,
number of test vectors $n_t$,
maximum failure probability $\varepsilon_{\text{algofail}}$

**Output:** local space $\Lambda^n_{\text{rand}}$ with property
$P(\|P_h - \text{proj}_{\Lambda^n_{\text{rand}}} P_h\| \leq \texttt{tol}) > (1 - \varepsilon_{\text{algofail}})$

`// initialize basis and test vectors`

2 $B \leftarrow \emptyset$

3 $M \leftarrow \left\{P_h\, D_{out}^{-1}\, \underline{\mathrm{M}}_{out}^{-1/2}\, \underline{\mathrm{r}}_1, \ldots, P_h\, D_{out}^{-1}\, \underline{\mathrm{M}}_{out}^{-1/2}\, \underline{\mathrm{r}}_{n_t}\right\}$

`// determine error estimator factor`

4 $\varepsilon_{\text{testfail}} \leftarrow \varepsilon_{\text{algofail}} / N_{P_h}$

5 $c_{\text{est}} \leftarrow \left(\sqrt{2}\, \text{erf}^{-1}\left( \sqrt[n_t]{\varepsilon_{\text{testfail}}}\right)\right)^{-1}$

`// basis generation loop`

6 **while** $(\max_{t \in M} |||t|||_{in}) \cdot c_{\text{est}} >$ `tol` **do**

7 $\quad B \leftarrow B \cup (P_h\, D_{out}^{-1}\, \underline{\mathrm{M}}_{out}^{-1/2}\, \underline{\mathrm{r}})$

8 $\quad B \leftarrow \text{orthonormalize}(B)$

9 $\quad M \leftarrow \left\{t - \text{proj}_{\text{span}(B)}\, t \mid t \in M\right\}$

10 **return** $\Lambda^n_{\text{rand}} = \text{span}(B)$

To construct a suitable approximation $\Lambda^n_{\text{rand}}$ of the optimal local space $\Lambda^n$, we introduce the adaptive randomized Algorithm 1 (cf. [SM2]). The algorithm iteratively enhances $\Lambda^n_{\text{rand}}$ with applications of the discrete transfer operator $P_h$ to random functions until a certain convergence criterion is satisfied. To be more precise, in each loop in line 7 we consider a different realization of a standard normal random vector $\underline{\mathrm{r}} \in \mathbb{R}^{N_{out}}$. Then, we apply $\underline{\mathrm{M}}_{out}^{-1/2}$ to $\underline{\mathrm{r}}$[1] in order to obtain an improved norm estimator and an improved a priori estimate (cf. Theorem SM1 and the discussion in section SM4 in [SM2]). Next, we introduce the mapping $D_{out}^{-1}$, which maps a coefficient vector in $\mathbb{R}^{N_{out}}$ to the corresponding FE function on $I \times \partial\Omega^{out}$ and apply this mapping to the vector $\underline{\mathrm{M}}_{out}^{-1/2}\, \underline{\mathrm{r}} \in \mathbb{R}^{N_{out}}$. Finally, we apply the discrete transfer operator $P_h$, meaning we solve the PDE locally on $I \times \Omega^{out}$ with boundary condition $D_{out}^{-1}\, \underline{\mathrm{M}}_{out}^{-1/2}\, \underline{\mathrm{r}}$ and restrict the solution to $I \times \Omega^{in}$. The restricted solution is added to the current basis, which is then orthonormalized using the numerically stable Gram-Schmidt with adaptive re-iteration from [SM1] as suggested in [SM2]. The loop terminates if the following probabilistic norm estimator is below the prescribed tolerance `tol`.

**Proposition SM1.** *(Probabilistic a posteriori norm estimator) Let $n_t$ realizations $\underline{r}_1, \ldots, \underline{r}_{n_t} \in \mathbb{R}^{N_{out}}$ of a standard normal random vector and the failure probability $\varepsilon_{\text{testfail}}$ be given. Then, the probabilistic a posteriori estimator*

$$\Delta(P_h - \text{proj}_{\Lambda^n_{rand}} P_h, n_t, \varepsilon_{\text{testfail}}) := c_{\text{est}}(n_t, \varepsilon_{\text{testfail}}) \max_{i=1,\ldots,n_t} |||(P_h - \text{proj}_{\Lambda^n_{rand}} P_h)\, D_{out}^{-1}\, \underline{M}_{out}^{-1/2}\, \underline{r}_i\, |||_{in}$$

[1]In practice we use the Cholesky decomposition $\underline{\mathrm{L}}\,\underline{\mathrm{L}}^\top$ of $\underline{\mathrm{M}}_{out}$ and apply $\underline{\mathrm{L}}^{-\top}$ to $\underline{\mathrm{r}}$ since the application of the inverse square root may be computationally expensive.

*is an upper bound for the norm* $\|P_h - \mathrm{proj}_{\Lambda^n_{rand}} P_h\|$ *with probability greater than or equal to* $(1 - \varepsilon_{\text{testfail}})$*, where* $c_{\text{est}}(n_t, \varepsilon_{\text{testfail}}) := 1/(\sqrt{2}\, erf^{-1}(\sqrt[n_t]{\varepsilon_{\text{testfail}}}))$*. Moreover, regarding the effectivity of the estimator, we have that*

$$P\left(\frac{\Delta(P_h - \mathrm{proj}_{\Lambda^n_{rand}} P_h, n_t, \varepsilon_{\text{testfail}})}{\|P_h - \mathrm{proj}_{\Lambda^n_{rand}} P_h\|} \leq c_{\text{eff}}(n_t, \varepsilon_{\text{testfail}})\right) \geq 1 - \varepsilon_{\text{testfail}}, \quad where$$

$$c_{\text{eff}}(n_t, \varepsilon_{\text{testfail}}) := \Big(Q^{-1}\Big(\frac{\mathrm{rank}(P_h - \mathrm{proj}_{\Lambda^n_{rand}} P_h)}{2}, \frac{\varepsilon_{\text{testfail}}}{n_t}\Big)\big(erf^{-1}(\sqrt[n_t]{\varepsilon_{\text{testfail}}})\big)^{-2}\Big)^{1/2}.$$

*Here,* $Q^{-1}$ *is the inverse of the upper normalized incomplete gamma function, which means that* $Q^{-1}(a, y) = x$ *if* $Q(a, x) = y$*.*

*Proof.* See proof of Proposition 3.7, 3.8, and SM4.3 in [SM2]. □

For the calculation of $c_{\text{est}}(n_t, \varepsilon_{\text{testfail}})$ in line 5 the rank $N_{P_h}$ of the discrete transfer operator $P_h$ is required. Since $N_{P_h}$ is unknown in practice, we use $\min\{N_{in}, N_{out}\}$ as an upper bound for $N_{P_h}$. Note that after $N_{P_h}$ steps we can infer that $\Lambda^n_{\text{rand}} = \mathrm{range}(P_h)$, consequently $\|P_h - \mathrm{proj}_{\Lambda^n_{\text{rand}}} P_h\| = 0$ and the algorithm terminates. Since the norm estimator is therefore executed at most $N_{P_h}$ times and the probability for one estimate to fail is $\varepsilon_{\text{testfail}}$, an union bound argument yields that the failure probability for the whole algorithm is $\varepsilon_{\text{algofail}} \leq N_{P_h}\, \varepsilon_{\text{testfail}}$.

The following probabilistic a priori error bound shows that the convergence behavior of the reduced approximation space $\Lambda^n_{\text{rand}}$ is quasi-optimal and only slightly worse than the rate $\sqrt{\lambda_{n+1}}$ achieved by the optimal local reduced space $\Lambda^n$.

**Proposition SM2.** *(Probabilistic a priori error bound) Let* $\lambda^{in}_{min}$ *and* $\lambda^{in}_{max}$ *denote the smallest and largest eigenvalue of the inner product matrix* $\underline{M}_{in}$*. Moreover, let* $\Lambda^n_{rand}$ *be the approximation space generated by Algorithm 1. Then, for* $n \geq 4$ *the following probabilistic a priori error bound holds*

$$\mathbb{E}(\|P_h - \mathrm{proj}_{\Lambda^n_{rand}} P_h\|) \leq \sqrt{\frac{\lambda^{in}_{max}}{\lambda^{in}_{min}}} \min_{\substack{k+p=n \\ k\geq 2, p\geq 2}} \left(\left(1 + \sqrt{\frac{k}{p-1}}\right)\sqrt{\lambda_{k+1}} + \frac{e\sqrt{n}}{p}\sqrt{\sum_{j>k} \lambda_j}\right).$$

*Proof.* See proof of Proposition 3.2 and SM4.2 in [SM2], which are based on [SM3]. □

## SM3. Global randomized GFEM algorithm

Exploiting the global a priori error bound and the local randomized adaptive basis generation algorithm (cf. Proposition 5.4 and Algorithm 1), the following global GFEM algorithm enables a localized construction of the local ansatz spaces such that the global GFEM approximation satisfies a desired global error tolerance with a very low failure probability. For more details regarding the computational realization of the global GFEM approximation see subsection 5.2.

In lines 2 to 6 we first calculate the local target accuracies $\texttt{tol}_i$ from the global target accuracy $\texttt{tol}_{\text{GFEM}}$ by exploiting the global a priori error bound in Proposition 5.4. The reduced inf-sup constant $\beta$ is the only global constant. However, the results in Table 1 in subsection 6.2 show that $\beta$ is close to one for our numerical experiments. Therefore, we can, for instance, either estimate $\beta$ by one or calculate the constant iteratively while increasing the number of ansatz and test functions and use the result as a regular update in the algorithm. Note that the latter option increases computational costs and we chose the former option in our numerical experiments (cf. subsection 6.2).

**Algorithm 2:** GFEM

1 **Function** `GFEM`($\texttt{tol}_{\text{GFEM}}$, $\varepsilon_{\text{fail}}$, $n_t$):

**Input :** target accuracy $\texttt{tol}_{\text{GFEM}}$, maximum failure probability $\varepsilon_{\text{fail}}$, number of test vectors $n_t$

**Output:** global approximation $u_h^{\text{GFEM}}$ with property

$$P\left(\frac{\sqrt{\|(u_h-u_h^{\text{GFEM}})_t\|^2_{L^2(I\times\Omega)}+\|\alpha^{\frac{1}{2}}\nabla(u_h-u_h^{\text{GFEM}})\|^2_{L^2(I\times\Omega)}}}{\|\alpha^{\frac{1}{2}}\nabla u_h\|_{L^2(I\times\Omega)}+\|f\|_{L^2(I\times\Omega)}+\|u_0\|_{L^2(\Omega)}+\|(u_h^b)_t\|_{L^2(I\times\Omega)}+\|\alpha^{\frac{1}{2}}\nabla u_h^b\|_{L^2(I\times\Omega)}} \leq \texttt{tol}_{\text{GFEM}}\right) \geq (1-\varepsilon_{\text{fail}})$$

`// calculate reduced inf-sup iteratively or use estimate`

2 calculate $\beta$

3 **for** $i \in \{1,\dots,M\}$ **do**

`// calculate local target accuracy`

4 calculate $c^{\alpha}_{p,i}$, $c_{f,i}$

5 $\max_i \leftarrow \max\left\{\left(1+\frac{1}{\beta}\right)\left[2M^{in}\left(c_1^2+\left(\frac{c_2\, c^{\alpha}_{p,i}}{\operatorname{diam}(\Omega_i^{in})}\right)^2\right)\right]^{\frac{1}{2}}, \frac{1}{\beta}\left(c_1+\frac{c_2}{\operatorname{diam}(\Omega_i^{in})}\right)\right\}$

6 $\texttt{tol}_i \leftarrow \texttt{tol}_{\text{GFEM}} \cdot \left(\sqrt{10\,M^{out}}\,\max\{2, c_{f,i}\}\max_i\right)^{-1}$

`// determine local proportion of global failure probability`

7 $\varepsilon_{\text{algofail}} \leftarrow \varepsilon_{\text{fail}}/M$

`// invoke adaptive randomized local basis generation`

8 $\Lambda^n_{\text{rand},i} \leftarrow$ `AdaptiveRandomizedLocalBasis`$(P_{h,i}, \texttt{tol}_i, n_t, \varepsilon_{\text{algofail}})$

`// enrich local reduced space with` $u^f_{h,i}|_{I\times\Omega_i^{in}}$ `and` $u^b_h|_{I\times\Omega_i^{in}}$

9 $\Lambda^{n,\text{data}}_{\text{rand},i} \leftarrow \Lambda^n_{\text{rand},i} \oplus \operatorname{span}(u^f_{h,i}|_{I\times\Omega_i^{in}})$

10 **if** $\partial\Omega_i^{out} \cap \partial\Omega \neq \emptyset$ **then**

11 $\Lambda^{n,\text{data}}_{\text{rand},i} \leftarrow \Lambda^{n,\text{data}}_{\text{rand},i} \oplus \operatorname{span}(u^b_h|_{I\times\Omega_i^{in}})$

`// construct global GFEM space and test space`

12 $X_h^{\text{GFEM}} \leftarrow \oplus_{i=1,\dots,M}\{\psi_i w_i \mid w_i \in \Lambda^{n,\text{data}}_{\text{rand},i}\}$

13 $V_h^{\text{GFEM}} \leftarrow \operatorname{proj}_{L^2(I,V)} X_h^{\text{GFEM}}$

`// solve reduced global problem`

14 find $u_h^{\text{GFEM}} \in X_h^{\text{GFEM}}$ such that

15 $\langle (u_h^{\text{GFEM}})_t, v_h\rangle + (\alpha\nabla u_h^{\text{GFEM}}, \nabla v_h) = \langle f, v_h\rangle$ for all $v_h \in V_h^{\text{GFEM}}$

16 **return** $u_h^{\text{GFEM}}$

Using the precalculated local target accuracies $\texttt{tol}_i$ and the local failure probabilities $\varepsilon_{\text{algofail}}$ we employ Algorithm 1 to construct local ansatz spaces in line 8. Subsequently, the local spaces are enriched with data correctors[2] in lines 9 to 11. Finally, the global reduced Petrov-Galerkin GFEM solution is computed in line 15 and thanks to the construction procedure the global GFEM approximation error satisfies the global target accuracy $\texttt{tol}_{\text{GFEM}}$ with failure probability $\varepsilon_{\text{fail}}$.

[2]Here, $u^f_{h,i}$ and $u^b_h$ denote the discrete counterparts of the data correctors $u^f_i$ and $u^b$ introduced in subsections 3.1 and 3.2

## References

[SM1] A. Buhr, C. Engwer, M. Ohlberger, and S. Rave, *A numerically stable a posteriori error estimator for reduced basis approximations of elliptic equations*, in Proceedings of the 11th World Congress on Computational Mechanics, X. O. E. Onate and A. Huerta, eds., CIMNE, Barcelona, 2014, pp. 4094–4102.

[SM2] A. Buhr and K. Smetana, *Randomized local model order reduction*, SIAM J. Sci. Comput., 40 (2018), pp. A2120–A2151.

[SM3] N. Halko, P. G. Martinsson, and J. A. Tropp, *Finding structure with randomness: probabilistic algorithms for constructing approximate matrix decompositions*, SIAM Rev., 53 (2011), pp. 217–288.

Institute for Computational and Applied Mathematics, University of Münster, Einsteinstr. 62, 48149 Münster, Germany, julia.schleuss@uni-muenster.de.

Department of Applied Mathematics, University of Twente, P.O. Box 217, 7500 AE Enschede, The Netherlands, k.smetana@utwente.nl.
